# Supplementary material for: EdgeRAG: Online-Indexed RAG for Edge Devices
Source: arXiv:2412.21023 source file (2024-12-31)
Supplement: Supplementary file 1 [file appendix.tex]

\todo{Move to appendix, Need help with the formalization}
Retrieval with Adaptive Cost-aware Caching's minimum caching threshold algorithm\\
Our objective is to minimize an expected retrieval latency\\
Let $E[x]$ is expected value of $x$,\\
$P[x]$ is the probability of $x$, and\\
$L[x]$ is the latency of $x$.\\
$H$, $M$, $NC$ are cache hit, cache miss, no-cache event respectively.\\
$Cache$ is a cache access event.\\
$E[latency] = P(H)L(H)+P(M)L(M)+P(NC)L(NC)$\\
First, let's take a look at the non-cache $P(NC)L(NC)$ term.\\
We already know the $L(NC)$ term from the initial indexing process (as shown in Figure \ref{fig:embed_gen_cost}).
However, we do not know the probability distribution of second-level cluster accesses. We make an initial assumption that second-level clusters are uniformly accessed.
Thus, $P(NC)$ follows that of the probability distribution function (PDF) of the embedding generation latency and 
we can find $P(NC)L(NC)$ by finding an integral of the PDF of embedding generation latency from 0 up to the minimum cluster embedding generation cost threshold.\\
Figure \ref{} \todo{add fig} shows the value of $P(NC)L(NC)$ as a function of the minimum cluster embedding generation cost threshold.\\
Next, we take a look at the cache miss $P(M)L(M)$ term.\\
Similar to $P(NC)L(NC)$ term, we can estimate the value of $P(M)L(M)$ using the PDF of the embedding generation latency.
However, because $1 = cache hit rate + cache miss rate$
\todo{Cost*}
